# Supplementary material for: SAMwave: Wavelet-Driven Feature Enrichment for Effective Adaptation of Segment Anything Model
Source: arXiv:2507.20186 source file (2025-07-27)
Supplement: Supplementary file 1 [file 6_supple.tex]

\clearpage
\setcounter{page}{1}
\maketitlesupplementary

\section{Additional Results}

\subsection{Quantitative Results}
\label{sec:quant}
As mentioned in the main manuscript, we provide quantitative results of SAMWave with SAM2 as the backbone for defocus blur detection, shadow detection, and forgery detection. We show their quantitative comparison in Tab.~\ref{tab:blur}, \ref{tab:shadow}, and \ref{tab:forgery}, respectively.
In defocus blur and shadow detection, we see performance significant performance gain across multiple datasets. However, for forgery detection, unlike the SAM backbone, we did not see any improvement over previous methods. Similar to EVP, our method also lags behind task-specific methods.

% \subsection{Qualitative Results}
% \label{sec:qual}
% We also provide qualitative results of camouflaged object detection in Fig.~\ref{fig:cod}.

% \begin{figure*}
%     \centering
%     \includegraphics[width=\linewidth]{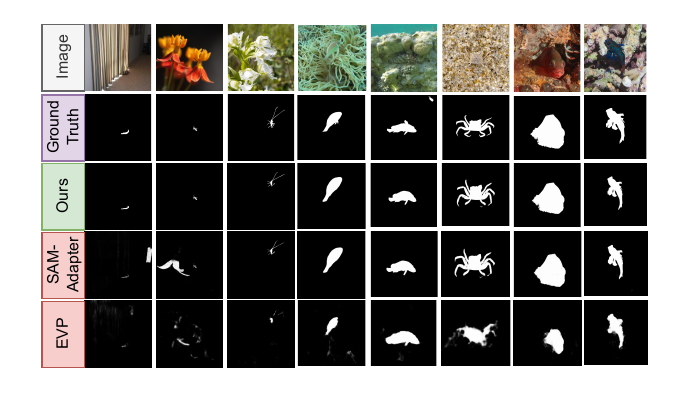}
%     \caption{Qualitative results of camouflaged object detection of our method compared with existing methods. As expected, both the SAM-adapter and EVP performed worse than our method. }
%     \label{fig:cod}
% \end{figure*}

\begin{table}[t]
\centering
      \caption{Comparison with state-of-the-art approaches on defocus blur detection for SAM2 backbone. The best result is shown in \textbf{bold}, and the second best is \underline{underlined}.}
      \centering
    \resizebox{0.8\columnwidth}{!}{
        \begin{tabular}{lcc|cc}
        \toprule
        \multirow{2}{*}{Method} & \multicolumn{2}{c|}{DUT} & \multicolumn{2}{c}{CUHK} \\
                                & $\mathcal{F}_{\beta} \uparrow$    & $\mathcal{M} \downarrow$   & $\mathcal{F}_{\beta} \uparrow$    & $\mathcal{M} \downarrow$ \\ \midrule
          DeFusionNet$^{(2019)}$\cite{DBLP:conf/cvpr/TangZLWZ19}                      & 0.823      & 0.118     & 0.818      & 0.117     \\
          BTBNet$^{(2018)}$\cite{DBLP:conf/cvpr/ZhaoZ0L18}                      & 0.827      & 0.138     & 0.889      & 0.082     \\
          CENet$^{(2019)}$\cite{DBLP:conf/cvpr/ZhaoZLL19}                      & 0.817      & 0.135     & 0.906      & 0.059     \\
          DAD$^{(2021)}$ \cite{DBLP:conf/cvpr/ZhaoSL21}                     & 0.794      & 0.153     & 0.884      & 0.079     \\
          EFENet$^{(2021)}$\cite{DBLP:journals/tip/ZhaoHHL21}                      & 0.854      & 0.094     & 0.914      & 0.053     \\
          EVP$^{(2023)}$\cite{DBLP:conf/cvpr/LiuSPC23}                      & {0.890}      & \underline{0.068}     & \textbf{0.928}      & 0.045     \\ 
          \midrule
          \multicolumn{5}{l}{\textbf{Real-valued Adapters}} \\ 
    \midrule
          Ours (daubechies)                      & \textbf{0.896}     & \textbf{0.051}     & 0.923      & \textbf{0.036}     \\
          Ours (coiflet)                     & 0.893      & \textbf{0.051}     & 0.924      & 0.039     \\
          Ours (haar)                     & \underline{0.894}      & \textbf{0.051}     & \underline{0.925}      & \underline{0.037}     \\
          Ours (symlet)                     & 0.893      & \textbf{0.051}     & 0.924      & 0.038 \\
          \midrule
          \multicolumn{5}{l}{\textbf{Complex-valued Adapters}} \\ 
          \midrule
          Ours (Symmetric-b)   & -  &  -   & - & -     \\
          Ours (Symmetric-a)   & -     & -     & 0.911     & 0.053     \\ \midrule
          \bottomrule
        \label{tab:blur}
        \end{tabular}
        }
\end{table}

\begin{table}
      \centering
        \caption{Comparison with state-of-the-art approaches on shadow detection on SAM2 backbone. The best result is shown in \textbf{bold}, and the second best is \underline{underlined}.}
        \resizebox{0.6\columnwidth}{!}{
        \begin{tabular}{lc|c}
        \toprule
        \multirow{2}{*}{Method} & ISTD & SBU \\
                                & BER $\downarrow$   & BER $\downarrow$ \\ \midrule
         Stacked CNN$^{(2016)}$\cite{DBLP:conf/eccv/VicenteHYHS16}      & 8.60      &  -      \\
         BDRAR$^{(2018)}$\cite{DBLP:conf/eccv/ZhuDHFXQH18}            & 2.69      & 3.89    \\
         DSC$^{(2018)}$\cite{DBLP:conf/cvpr/Hu0F0H18}              & 3.42      & 5.59    \\
         DSD$^{(2019)}$\cite{DBLP:conf/cvpr/ZhengQCL19}              & 2.17      & 3.45    \\
         FDRNet$^{(2021)}$ \cite{DBLP:conf/iccv/Zhu0KL21}          & 1.55      & 3.04    \\
         MTMT$^{(2020)}$\cite{DBLP:conf/cvpr/Chen0WW0H20}             & 1.72      & 3.15    \\
         EVP$^{(2023)}$\cite{DBLP:conf/cvpr/LiuSPC23}              & 1.35      & 4.31    \\
         Sam-Adapter$^{(2023)}$\cite{chen2023sam}      & 1.43      & -       \\ 
         Sam2-Adapter$^{(2024)}$\cite{chen2024sam2adapterevaluatingadapting}     & 1.43      & -  \\
    \midrule
          \multicolumn{3}{l}{\textbf{Real-valued Adapters}} \\ 
          \midrule
         Ours (daubechies)            & 1.91 & \underline{3.04}        \\ 
         Ours (coiflet)            & 1.24 & 5.28        \\
         Ours (haar)                & \textbf{0.92} & \textbf{2.99}       \\
         Ours (symlet)                 & \underline{1.22} & 3.77        \\
             \midrule
          \multicolumn{3}{l}{\textbf{Complex-valued Adapters}} \\ 
          \midrule
          Ours (Symmetric-b)  & - & -       \\
          Ours (Symmetric-a)  & 1.32 & 4.32       \\
        \midrule \bottomrule
        \end{tabular}
        }
        \label{tab:shadow}
    \end{table}

\begin{table}
      \centering
        \caption{Comparison with existing methods on forgery detection on SAM2 backbone. The best result is shown in \textbf{bold}, and the second best is \underline{underlined}.}
        \resizebox{0.6\columnwidth}{!}{
        \begin{tabular}{lcc}
        \toprule
        \multirow{2}{*}{Method} & \multicolumn{2}{c}{IMD20} \\
                                & $\mathcal{F}1 \uparrow$    & AUC $\uparrow$   \\ 
        \midrule
         ManTra$^{(2019)}$\cite{DBLP:conf/cvpr/0001AN19}               & -      & 0.748     \\
         SPAN$^{(2020)}$\cite{DBLP:conf/eccv/HuZJCYN20}                & -      & 0.750         \\
         PSCCNet$^{(2022)}$\cite{liu2022pscc}                          & -      & 0.806         \\
         TransForensics$^{(2021)}$\cite{DBLP:conf/iccv/HaoZYXP21}      & -      & \textbf{0.848}         \\
         ObjectFormer$^{(2022)}$\cite{DBLP:conf/cvpr/WangWCHSLJ22}     & -      & \underline{0.821}         \\
         EVP$^{(2023)}$\cite{DBLP:conf/cvpr/LiuSPC23}                  & \textbf{0.443}  & {0.807}         \\ 
     \midrule
         Ours (daubechies)         &   0.132      & 0.500           \\ 
         Ours (coiflet)            &   \underline{0.416}      & 0.658           \\
         Ours (haar)               &  0.131      & 0.499    \\
         Ours (symlet)             &   0.372      & 0.686    \\
         \bottomrule
        \end{tabular}
        }
        \label{tab:forgery}
    \end{table}
